# Supplementary material for: Unusual Diffusivity in Strongly Disordered Quantum Lattices: Random Dimer Model
Source: arXiv:2405.20813 ancillary file (2024-05-31)
Supplement: Supplementary file 1 [file sup-mat.pdf]

# Supplementary Material
# "Unusual Diffusivity in Strongly Disordered Quantum Lattices: Random Dimer Model"

Ilia Tutunnikov[1,2] and Jianshu Cao[1,*]
[1] Department of Chemistry, Massachusetts Institute of Technology, 77 Massachusetts Avenue, Cambridge, Massachusetts 02139, USA
[2] ITAMP, Center for Astrophysics | Harvard & Smithsonian, Cambridge, Massachusetts 02138, USA

This Supplementary Material summarizes the main steps in the derivations of equations presented in the main text. Additionally, several supporting figures are presented.

## CONTENTS

I. $W(\sigma)$ scaling 1

II. Random dimer model 1
A. $D(t)$ near the turnover 2

III. Dimer in presence of noise 2
A. Asymptotic formula, first term 2
B. Asymptotic formula, second term 3

IV. Haken-Strobl-Reineker model in the eigenbasis representation 3

References 4

## I. $W(\sigma)$ SCALING

The width of the stationary probability distribution (or the localization length) in the weak disorder regime can be estimated as follows. The dispersion relation in a nearly ordered section of a lattice with nearest-neighbor coupling is $E(k) \approx 2J\cos(k)$, where $k = 2\pi n/L$, and $L$ is the length of the section (i.e., localization length). For typical states in the center of the band, $\delta E = \partial_k E(k)|_{k=\pi/2}\delta k = 2J(2\pi/L)$. Disorder introduces energy fluctuations, and the ensemble averaged fluctuation is $\langle(\Delta E)^2\rangle = \sigma^2/L$. Localization occurs when $(\delta E)^2 = \langle(\Delta E)^2\rangle \implies L \propto J^2/\sigma^2$. In the strong disorder regime, the typical energies can be estimated as $\delta E = E(n=1) - E(n=0) \propto J/L^2$, while the energy fluctuation is $\sqrt{\langle(\Delta E)^2\rangle} \propto \sigma$. Thus, $\delta E = \sqrt{\langle(\Delta E)^2\rangle} \implies L \propto \sqrt{J/\sigma}$. These scalings are consistent with the scalings in Fig. 1 in the main text.

We can also explicitly calculate the variance of dimer eigenstates

$$W^2_{dimer} = \frac{4J^2}{4J^2 + (\Delta \pm \sqrt{4J^2+\Delta^2})^2} - \left[\frac{4J^2}{4J^2 + (\Delta \pm \sqrt{4J^2+\Delta^2})^2}\right]^2, \quad (1)$$

where $\Delta$ is the energy difference between the two sites. Ensemble-averaged $W^2_{dimer}$ reads

$$\langle W^2_{dimer}(\sigma)\rangle = \frac{\sqrt{\pi}J^2}{4\sigma|J|} e^{J^2/\sigma^2} \mathrm{erfc}\left(\frac{|J|}{\sigma}\right) \propto \frac{1}{\sigma}. \quad (2)$$

Figure 1 shows the numerically evaluated stationary state width, $W(\sigma)$. The scaling is close to $\sigma^{-1/2}$ – the scaling of $\sqrt{\langle W^2_{dimer}\rangle}$. Moreover, the asymptotic diffusivity of a random dimer $D_A \propto \sigma^{-1}$, which implies $W \propto \sqrt{\langle n^2\rangle} \propto \sqrt{\int D_A(t)\,dt} \propto \sigma^{-1/2}$.

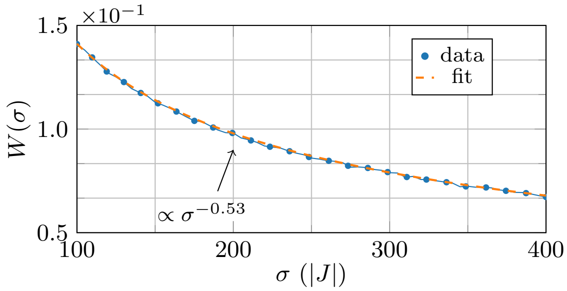


FIG. 1. Numerically calculated stationary state width as a function of disorder stregth, $\sigma$.

## II. RANDOM DIMER MODEL

In this section, we detail the derivation of the asymptotic formula for the diffusivity in a random dimer. To evaluate the integral:

$$D(t) = \frac{2J^2}{2\sigma\sqrt{\pi}}\mathrm{Im}\left[\int_{-\infty}^{\infty} \frac{\exp\left(it\sqrt{4J^2+\epsilon_{01}^2}\right)}{\sqrt{4J^2+\epsilon_{01}^2}} \times \exp\left(-\frac{\epsilon_{01}^2}{4\sigma^2}\right) d\epsilon_{01}\right]. \quad (3)$$

we use the method of stationary phase. Expanding the argument of the exponential in a Taylor series (up to and including terms $\propto \epsilon_{01}^2$) at the stationary point $\epsilon_{01} = 0$ allows to evaluate the integral

$$D_A(t) \sim \frac{J^2}{\sigma\sqrt{\pi}}\mathrm{Im}\left[\exp\left(\frac{J^2 - 3i|J|t\sigma^2}{2\sigma^2}\right) K_0\left(\frac{J^2 + i|J|t\sigma^2}{2\sigma^2}\right)\right] \approx \frac{J^2}{\sigma\sqrt{\pi}}\mathrm{Im}\left[\exp(-3i|J|t/2)K_0(i|J|t/2)\right] \quad (4)$$

where $K_0$ is the modified Bessel function of order zero. In the second line, we neglected terms $\propto \sigma^{-2}$ in the arguments of exponential and Bessel functions. Using the asymptotic formula for $K_0$ at large $t$, we arrive at

$$D_A(t) \sim \frac{|J|^{2/3}}{\sigma} \frac{\sin(2|J|t + \pi/4)}{\sqrt{t}}. \quad (5)$$

Figure 2 shows two examples where the time dependent diffusivity in a chain is compared to $D_A(t)$.

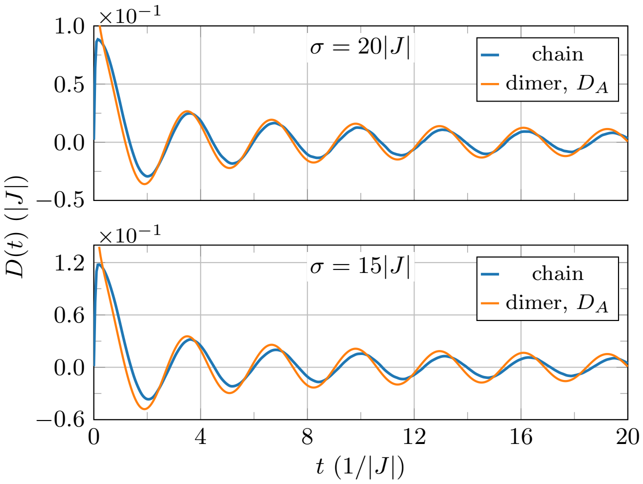


FIG. 2. Diffusivity in a chain vs $D_A(t)$ in Eq. (5).

### A. $D(t)$ near the turnover

Next, we focus on the behavior of $D(t)$ near the turnover. Expanding $\dot{P}_1(t)$ in in a Taylor series (up to and including terms $\propto J^4$), we get

$$\begin{aligned} D(t) &= \frac{1}{2\sigma\sqrt{\pi}} \int_{-\infty}^{\infty} \dot{P}_1(t) \exp\left(-\frac{\epsilon_{01}^2}{4\sigma^2}\right) d\epsilon_{01} \\ &\approx \frac{\sqrt{\pi}J^2}{\sigma}(1 - J^2t^2)\mathrm{erf}(\sigma t) - \frac{J^4}{\sigma^2} e^{-\sigma^2 t^2} t + \frac{\sqrt{\pi}J^4}{2\sigma^3}\mathrm{erf}(\sigma t) \\ &\approx \frac{\sqrt{\pi}J^2}{\sigma}(1 - J^2t^2)\mathrm{erf}(\sigma t), \ \sigma \gg |J| \end{aligned} \tag{6}$$

For the turnover time, we consider the derivative

$$\dot{D}(t) = 2J^2 e^{-\sigma^2 t^2} - \frac{2\sqrt{\pi}J^4}{\sigma}\mathrm{erf}(\sigma t)t. \tag{7}$$

$$\implies t_p = \frac{1}{\sqrt{2}\sigma}\sqrt{\mathrm{ProductLog}\left(\frac{2\sigma^4}{\pi J^4}\right)}, \tag{8}$$

where ProductLog is the Lambert $W$ function. For $\sigma \gg |J|$, the turnover point is given by

$$t_p \sim \frac{1}{\sigma\sqrt{2}}\sqrt{\ln\left(\frac{2\sigma^4}{\pi J^4}\right) - \ln\left[\ln\left(\frac{2\sigma^4}{\pi J^4}\right)\right]}, \tag{9}$$

where we used the asymptotic formula for large argument of product log function.

## III. DIMER IN PRESENCE OF NOISE

In this section, we consider the dimer in the presence of HSR noise. The density matrix elements satisfy the following set of differential equations

$$\begin{aligned} \dot{\rho}_{11}(t) &= -iJ(\rho_{12} + \rho_{21}), \\ \dot{\rho}_{12}(t) &= -(\Gamma - i\epsilon_{01})\rho_{12} - iJ(\rho_{22} - \rho_{11}), \\ \dot{\rho}_{21}(t) &= -(\Gamma + i\epsilon_{01})\rho_{12} - iJ(\rho_{11} - \rho_{22}), \\ \dot{\rho}_{22}(t) &= -iJ(\rho_{12} - \rho_{21}). \end{aligned} \tag{10}$$

These equations can be solved by the Laplace transform method. In the Laplace space, the population of site $n = 1$ is given by

$$P_1(s) = \frac{2J^2(\Gamma + s)}{s(s-\omega_1)(s-\omega_2)(s-\omega_3)}, \tag{11}$$

where $\omega_1$, $\omega_2$, and $\omega_3$ are the roots of the cubic polynomial

$$p(s) = s^3 + 2\Gamma s^2 + (\Gamma^2 + \epsilon_{01}^2 + 4J^2)s + 4\Gamma J^2. \tag{12}$$

Applying the inverse Laplace transform, we recover $P_1(t)$, and the diffusivity is given by

$$\begin{aligned} D^{HSR}(t) = \dot{P}_1(t) &= \frac{2J^2(\Gamma + \omega_1)e^{\omega_1 t}}{(\omega_1 - \omega_2)(\omega_1 - \omega_3)} \\ &+ \frac{2J^2(\Gamma + \omega_2)e^{\omega_2 t}}{(\omega_2 - \omega_1)(\omega_2 - \omega_3)} + \frac{2J^2(\Gamma + \omega_3)e^{\omega_3 t}}{(\omega_3 - \omega_1)(\omega_3 - \omega_2)}. \end{aligned} \tag{13}$$

So far, the formula for $D^{HSR}(t)$ is exact. However, it involves the roots $\omega_1$, $\omega_2$, and $\omega_3$ of the cubic polynomial in Eq. (12). The exact formulas for the roots are quite cumbersome, thus we approximate them. The discriminant of $p(s)$ is negative for the whole range of $\epsilon_{01}$ and relevant values of $\Gamma$ ($\Gamma/|J| < 3$). Negative discriminant implies that the polynomial has one real, $\omega_1$ and two complex roots that are complex conjugates, i.e., $\mathrm{Re}[\omega_2] = \mathrm{Re}[\omega_3]$ and $\mathrm{Im}[\omega_2] = -\mathrm{Im}[\omega_3]$. Expanding the analytical formula for the real root $\omega_1$ up the first order in $\Gamma$ term, we get the approximation

$$\omega_1 \approx -\frac{4J^2\Gamma}{\epsilon_{01}^2 + 4J^2}. \tag{14}$$

Similarly,

$$\mathrm{Re}[\omega_2] \approx -\frac{\epsilon_{01}^2 + 2J^2}{\epsilon_{01}^2 + 4J^2}\Gamma, \quad \mathrm{Im}[\omega_2] \approx \sqrt{\epsilon_{01}^2 + 4J^2}. \tag{15}$$

### A. Asymptotic formula, first term

Next, we evaluate the ensemble averaged $D^{HSR}(t)$. Starting from the first term $\propto \exp(\omega_1 t)$, we consider only the leading in $\Gamma$ term of the exponential function prefactor, such that

$$\begin{aligned} D_1^{HSR}(t) = \frac{\Gamma J^2}{\sqrt{\pi}\sigma} \int_{-\infty}^{\infty} \frac{\epsilon_{01}^2}{(\epsilon_{01}^2 + 4J^2)^2} \exp\left[-\frac{4\Gamma J^2 t}{\epsilon_{01}^2 + 4J^2}\right] \\ \times \exp\left[-\frac{\epsilon_{01}^2}{4\sigma^2}\right] d\epsilon_{01}. \end{aligned} \tag{16}$$

To evaluate the integral for asymptotically large $t$, we expand the time-dependent exponential into a power series in $t$ and integrate term by term

$$\begin{aligned} D_1^{HSR}(t) = \sum_{n=0}^{\infty} \frac{\Gamma(J/\sigma)^{2n+2}(-\Gamma t)^n}{4n!} \\ \times \mathrm{HyperU}\left(n+2, n+\frac{3}{2}, \frac{J^2}{\sigma^2}\right), \end{aligned} \tag{17}$$

where HyperU is Tricomi confluent hypergeometric function. To obtain a more useful expression, we use the fact that in a strong disorder limit $J^2/\sigma^2 \ll 1$, and expand HyperU in a Taylor series. Considering only the first two terms in the series allows to evaluate the sum in Eq. (17)

$$D_1^{HSR}(t) \approx \frac{\sqrt{\pi}}{4}\Gamma\sqrt{\frac{J^2}{\sigma^2}}\left[I_0\left(\frac{t\Gamma}{2}\right)+I_1\left(\frac{t\Gamma}{2}\right)\right]e^{-\Gamma t/2} - \frac{J}{2\sigma}\sqrt{\frac{\Gamma}{t}}\sinh\left(\frac{2J\sqrt{\Gamma t}}{\sigma}\right), \quad (18)$$

where $I_0$ and $I_1$ are the modified Bessel functions of the first kind of order zero and one. Strictly, $D_1^{HSR}$ tends to zero as $t \to \infty$, however, due to the approximation of the HyperU function, the asymptotic behavior in Eq. (18) is incorrect. Nevertheless, the formula in Eq. (18) is an adequate approximation to the diffusivity of a random dimer in the considered time window as confirmed by Fig. 3. Moreover, we can roughly write

$$D_1^{HSR}(t) \sim \frac{|J|}{2\sigma}\sqrt{\frac{\Gamma}{t}} - \frac{J^2\Gamma}{\sigma^2}, \quad (19)$$

where we used the asymptotic formulas for $I_0$ and $I_1$.

### B. Asymptotic formula, second term

The second term of the ensemble averaged diffusivity is approximately given by

$$D_2^{HSR}(t) = -\frac{iJ^2e^{-\Gamma t}}{2\sqrt{\pi}\sigma}\int_{-\infty}^{\infty}\frac{\exp\left[-\epsilon_{01}^2/(4\sigma^2)\right]}{\sqrt{\epsilon_{01}^2+4J^2}} \times \exp\left[it\sqrt{\epsilon_{01}^2+4J^2}+\frac{2J^2\Gamma t}{\epsilon_{01}^2+4J^2}\right]d\epsilon_{01}. \quad (20)$$

where we keep only the $\Gamma$-*independent* terms outside the exponential function. To evaluate the integral, we proceed similar to Section II, and apply the method of stationary phase. Since the third term of the ensemble averaged diffusivity is complex conjugate of the second one, we can write

$$D_2^{HSR}(t)+D_3^{HSR}(t)=2\mathrm{Re}[D_2^{HSR}(t)] \sim \frac{\sqrt{2}J^2e^{-\Gamma t/2}}{\sigma\sqrt{t}(\Gamma^2+4J^2)^{1/4}}\sin\left[2t|J|-\frac{1}{2}\arg(\Gamma-2i|J|)\right]. \quad (21)$$

Notice that for $\Gamma \to 0$, the above expression reduces to Eq. (5). Overall, the asymptotic dimer diffusivity in the HSR model is $D_A^{HSR} = D_1^{HSR} + 2\mathrm{Re}[D_2^{HSR}(t)]$, where $D_1^{HSR}(t)$ and $D_2^{HSR}(t)$ are given by Eq. (18) [or Eq. (19)] and Eq. (21).

Figure 3 compares the exact and the approximate dimer diffusivities. The figure shows that for the strong disorder, $\sigma/|J| = 20$, the asymptotic formulas work exceptionally well for both decoherence rates, $\Gamma/|J| = 0.5, 1$.

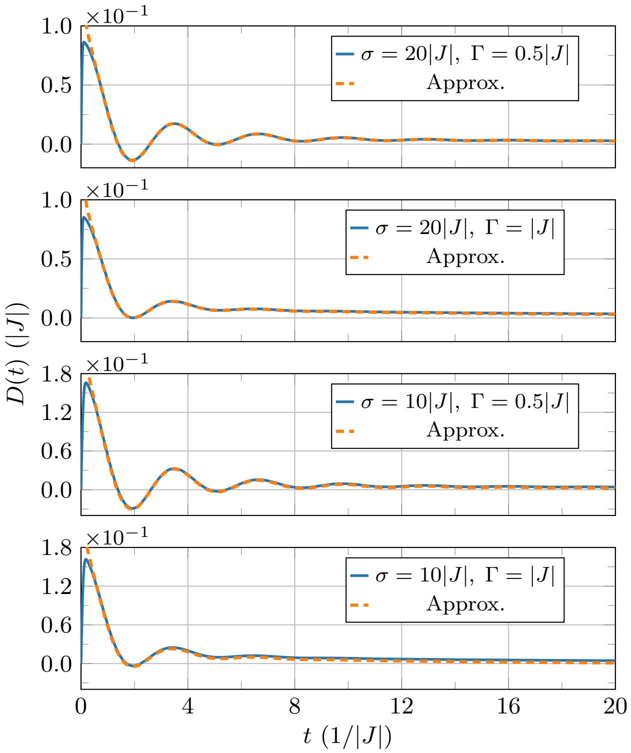


FIG. 3. Diffusivity in a HSR chain vs the asymptotic formulas in Eqs. (18) and (21).

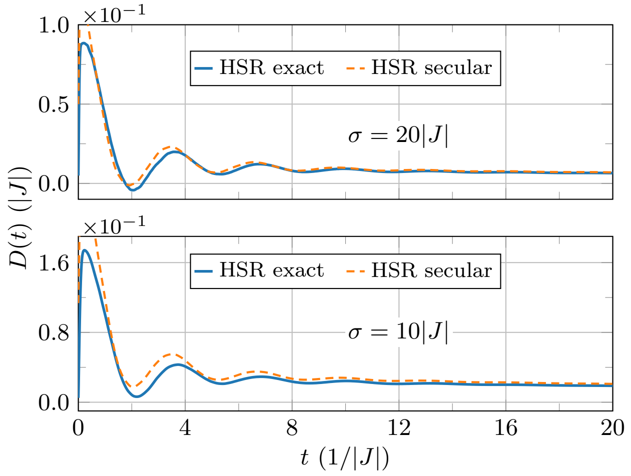


FIG. 4. Diffusivity in exact HSR model vs the secular approximation, see Eqs. (30) and (31). Here, $\Gamma = 0.5|J|$.

## IV. HAKEN-STROBL-REINEKER MODEL IN THE EIGENBASIS REPRESENTATION

In this section, we rewrite the Linblad master equation in the Haken-Strobl-Reineker (HSR) model in the eigenbasis of the quantum lattice. In the HSR model, the density matrix satisfied the following equation

$$\dot{\rho} = -i[H,\rho] - \frac{\Gamma}{2}\sum_n [V_n,[V_n,\rho]], \quad (22)$$

where the matrix elements of $V_n$ are $(V_n)_{j,k} = \delta_{j,n}\delta_{k,n}$, and $\Gamma$ is the rate of decoherence. We can rewrite Eq. (22) as

$$\dot{\rho} = -i[H,\rho] - \Gamma\rho_H, \quad (23)$$

where $\rho_H$ is a "hollow density matrix", with elements $(\rho_H)_{m,n} = (1-\delta_{m,n})\rho_{m,n}$.

Let $U$ be a unitary matrix with the eigenvectors of the Hamiltonian arranged in rows. The elements of the density matrix expressed in the eigenbasis, $\tilde{\rho}$ are obtained by the unitary trasnformation

$$\tilde{\rho} = U\rho U^{\dagger} \iff \tilde{\rho}_{i,j} = \sum_{m,n} U_{i,m}\rho_{m,n}U^{\dagger}_{n,j}, \quad (24)$$

where $\rho_{m,n}$ are the elements of the density matrix expressed in the site basis. Applying the orthogonal transformation to Eq. (23), we get

$$\begin{aligned}\dot{\tilde{\rho}}_{i,j} &= -i\omega_{i,j}\tilde{\rho}_{i,j} - \Gamma\sum_{m,n} U_{i,m}(1-\delta_{m,n})\rho_{m,n}U^{\dagger}_{n,j} \\ &= -i(\omega_{i,j} - i\Gamma)\tilde{\rho}_{i,j} + \Gamma\sum_{m,n} U_{i,m}\delta_{m,n}\rho_{m,n}U^{\dagger}_{n,j}, \end{aligned} \quad (25)$$

where $\omega_{i,j} = \omega_i - \omega_j$ is the difference of $j$-the and $k$-th eigeneneregies. The sum in the last term, $\sum_{m,n} U_{i,m}\delta_{m,n}\rho_{m,n}U^{\dagger}_{n,j} = \sum_m U_{i,m}\rho_{m,m}U^{\dagger}_{m,j}$ contains the diagonal elements of the density matrix expressed in the sites basis, $\rho_{m,m}$. To complete the transformation to the eigenbasis, we have to express $\rho_{m,m}$ in terms of elements of $\tilde{\rho}$, i.e.,

$$\rho_{m,m} = \sum_{k,l} U^{\dagger}_{m,k}\tilde{\rho}_{k,l}U_{l,m}. \quad (26)$$

Substitution yield the last term results in

$$\Gamma\sum_m U_{i,m}\rho_{m,m}U^{\dagger}_{m,j} = \sum_{m,k,l} U_{i,m}U^{\dagger}_{m,j}U^{\dagger}_{m,k}U_{l,m}\tilde{\rho}_{k,l}. \quad (27)$$

Overall, in the eigenbasis, density matrix elements satisfy the differential equation

$$\begin{aligned}\dot{\tilde{\rho}}_{i,j} &= -i(\omega_{i,j} - i\Gamma)\tilde{\rho}_{i,j} + \Gamma\sum_{k,l}\kappa^{(i,j)}_{k,l}\tilde{\rho}_{k,l}, \\ \kappa^{(i,j)}_{k,l} &= \sum_m U_{i,m}U^{\dagger}_{m,j}U^{\dagger}_{m,k}U_{l,m}, \end{aligned} \quad (28)$$

The equation can be simplified considerably by applying the secular approximation [1–3]. Within this approximation, the off-diagonal elements satisfy the following equations

$$\begin{aligned}\dot{\tilde{\rho}}_{i,j} &= -i(\omega_{i,j} - i\Gamma)\tilde{\rho}_{i,j} + \Gamma\kappa^{(i,j)}_{i,j}\tilde{\rho}_{i,j}, \ i \neq j, \\ \kappa^{(i,j)}_{i,j} &= \sum_m U_{i,m}U^{\dagger}_{m,j}U^{\dagger}_{m,i}U_{j,m} = \sum_m |U_{i,m}|^2|U_{j,m}|^2 \end{aligned} \quad (29)$$

where we used $U^{\dagger}_{m,i} = U^{*}_{i,m}$. Thus,

$$\tilde{\rho}_{i.j} = \tilde{\rho}_{i,j}(0)e^{-i\omega_{ij}t}\exp\left[-\Gamma(1-\kappa^{(i,j)}_{i,j})t\right], \ i \neq j. \quad (30)$$

The diagonal elements satisfy

$$\begin{aligned}\dot{\tilde{\rho}}_{i,i} &= -\Gamma\tilde{\rho}_{i,i} + \Gamma\sum_j \kappa^{(i,i)}_{j,j}\tilde{\rho}_{j,j}, \\ \kappa^{(i,i)}_{j,j} &= \sum_m |U_{i,m}|^2|U_{j,m}|^2. \end{aligned} \quad (31)$$

Figure 4 compares the diffusivity obtained by a direct solution of Eq. (23) vs the diffusivity obtained from Eq. (30) and Eq. (31).

* jianshu@mit.edu

[1] A. Nitzan, *Chemical Dynamics in Condensed Phases* (Oxford University Press, 2006).
[2] L. Valkunas, D. Abramavicius, and T. Mančal, *Molecular Excitation Dynamics and Relaxation* (Wiley-VCH, 2013).
[3] J. M. Moix, M. Khasin, and J. Cao, Coherent quantum transport in disordered systems: I. The influence of dephasing on the transport properties and absorption spectra on one-dimensional systems, New J. Phys. **15**, 085010 (2013).
